# Supplementary material for: CRLLK: Constrained Reinforcement Learning for Lane Keeping in Autonomous Driving
Source: arXiv:2503.22248 source file (2025-03-28)
Supplement: Supplementary file 1 [file appendix.tex]

\section{Appendix}
\label{Appendix}

\subsection{Development environment}
We development our model on a single workstation equipped with an Intel(R) Xeon(R) Gold 5220R CPU (24 cores, 48 threads) with NVIDIA GeForce RTX 3090 GPU. The training environment is built on open source Pytorch docker image\footnote{https://hub.docker.com/r/pytorch/pytorch} and Duckietown RL simulator~\cite{paull2017duckietown}. The Duckietown simulator consists of a Duckiebot and a set of configurable lane-keeping scenarios for training the Duckiebot, which provides data sampling during training and algorithm verification in testing. The Duckiebot inputs RGB environment observations from a monocular camera, and outputs the action corresponding to the wheel speeds of the Duckiebot. With the default settings, the Duckietown simulation applies actions in a frame-rate of 30 Hz. Each frame represents approximately 33.3 milliseconds ($10^{-3}\ s$) in the simulation. While the simulator maintains consistent time progression, the actual execution time in real-world may vary depending on the computational resources.

%\aea{citation missing[Re: done]}. More details on the experiment setup are provided in supplementary materials. 

\subsection{Action space}
\label{Appendix_actionspace}
In the Duckietown framework, vehicle navigation is controlled by adjusting the speeds of the Duckiebot’s wheels, with the wheel-speed action values ranging from -1 to 1. This corresponds to a vehicle speed range of $-0.21$ to $0.21$ $m/s$ in the real-world physical representation. For a discrete action based agent, we use three actions same as~\cite{almasi2020robust} --- turn-left, turn-right, and go-straight. Each discrete action translates to an appropriate left and right wheel speed. The mapping is shown in Table~\ref{tab:actions}.
\begin{table}[h]
    \centering
    \caption{Wheel speeds of three different actions of discrete action space~\cite{almasi2020robust}. The range of each wheel speed is $[-1,1]$.}
    \begin{tabular}{lcc}
\hline
\textbf{Action} & \textbf{Left wheel} & \textbf{Right wheel} \\
\hline
turn-left & 0.04 & 0.4 \\
% \hline
turn-right & 0.4 & 0.04 \\
% \hline
go-straight & 0.3 & 0.3 \\
\hline
\end{tabular}
    \label{tab:actions}
\end{table}

For a continuous action based agent, the action space is represented as a 2-dimensional vector corresponding to the steering and speed actions of the Duckiebot. Both the steering and speed actions are ranging in $[-1,1]$, mapping to $[-\pi,\pi]$ for steering direction and $[-0.21,0.21]\ m/s$ for driving speed of the Duckiebot. We model network-based policy outputs using a 2D multivariate Gaussian distribution for steering angle and speed. The outputs of the action mean $(\mu)$ and the standard deviation $(\sigma)$ allow for sampling steering and speed actions from a 2D multivariate action distribution. The mean employs the $\mathrm{tanh}$ activation function to bound the action mean between $(-1,1)$, while the standard deviation utilizes the $\mathrm{sigmoid}$ activation function with a clamped value between $(0.2,0.6)$ to balance between exploration and exploitation.

\subsection{Detailed description of training}
The algorithm training code employs a distributed AI framework Ray~\cite{moritz2018ray} to speed up the training process through higher data collection efficiency. Four distributed nodes work in parallel remotely for the agent's trajectory collection, while one global node is responding to update the network and the Lagrange parameters using the collected trajectory buffer. After collecting trajectory buffers from distributed nodes, the actor network is trained by PPO~\cite{schulman2017proximal}, and the critic network is updated by Mean Square Error (MSE) algorithm.

\vskip 2pt
\noindent{\textbf{Hyper-parameters:}} Key hyper-parameters include a maximum episode length of $H=512$ and a discount factor $\gamma=0.95$. The learning rates for the policy and Lagrangian multipliers are set as $\eta_{3}=\eta_{2}=\eta_{1}=2e^{-5}$, while the critic's learning rate is $\eta_{4}=1e^{-5}$. All hyper-parameters of experiment are listed in Table \ref{tab:parameters}. 

\vskip 2pt
\noindent{\textbf{Baselines:}}
The learning rate for the actor-critic network ($\eta_3$) and that for language multipliers ($\eta_1, \eta_2$) are fixed to the same value as $2e^{-5}$. 
\begin{table}[t]
    \centering
    \caption{Hyper-parameters involved in our experiment.}
    \begin{tabular}{lcl}
\toprule
\textbf{Parameters} & \textbf{Value} & \textbf{Description} \\
\midrule
$\eta$ & 2e-5 & Learning rate for gradient decent.\\
Runner & 4 & Parallel threads for data sampling.\\
$H$ & 512 & Batch size and the episode length.\\
$\gamma$& 0.95 &  Discount factor in RL.\\
$\epsilon$& 0.2 & Clip factor for PPO algorithm.\\
$\alpha_{1}$& 0.5 & Constrain threshold for lane deviation.\\
$\alpha_{2}$& 0.02 & Constrain threshold for collision.\\
$\alpha_{3}$& 0.01 & Constrain threshold for illegal driving.\\
reward factor& 10 & Gain for travel distance cost in reward.\\ 
lane factor& 100 & Gain for lane distance cost in reward.\\
collision factor& 40 & Gain for collision cost in reward.\\
illegal factor& 10 & Gain for illegal driving in reward.\\
Gradient clip& 10 & Gradient clip factor.\\
$\sigma$ clip& (0.2,0.6) & Actor variance boundary.\\
entropy factor& 0.001 & Entropy factor for policy gradient.\\
\bottomrule
\end{tabular}

    \label{tab:parameters}
\end{table}
For the baseline methods \bl, \dppof\ and \cppof, we use the same coefficient combination as the previous RL approach~\cite{almasi2020robust}: 10 for travel distance reward, -100 for lane deviation cost, and –40 for every boundary collision as the actual leaving-track punishment in previous work~\cite{almasi2020robust}.
\begin{alignat*}{1}
\hat{r}(s_t,a_t) =  10r(s_t, a_t) - 100 \cl(s_t,a_t) - 40\cc(s_t,a_t) 
\end{alignat*}
To improve training efficiency and facilitate learning of smaller Lagrangian multipliers within a short time, we apply a weighting scheme from prior research~\cite{almasi2020robust}. Specifically, the Lagrangian multipliers are weighted in the reward function as follows:
\begin{alignat*}{1}
\hat{r}(s_t,a_t, \lambda_{1}, \lambda_{2}) =  10r(s_t, a_t) - 100\lambda_{1} \cl(s_t,a_t) - 40\lambda_{2} \cc(s_t,a_t) 
\end{alignat*}
where $\lambda_{1}, \lambda_{2}\equiv 1$ is the standard RL with fixed weight coefficient combination in prior research~\cite{almasi2020robust}. These cost gain factors speed up the convergence in practice by amplifying the multipliers, while not changing the essence of adaptive update.

% \noindent{\textbf{Hyper-parameters:}} Key hyper-parameters include a maximum episode length of $H=512$ and a discount factor $\gamma=0.95$. The learning rates for the policy and Lagrangian multipliers are set as $\eta_{3}=\eta_{2}=\eta_{1}=2e^{-5}$, while the critic's learning rate is $\eta_{4}=1e^{-5}$. To improve training efficiency and facilitate learning of smaller Lagrangian multipliers within a short time, we apply a weighting scheme from prior research~\cite{almasi2020robust}. Specifically, the Lagrangian multipliers are weighted in the reward function as follows:
% \begin{alignat*}{1}
% % \hspace{-0.2cm}
% \hat{r}(s_t,a_t, \lambda_{1}, \lambda_{2}) =  10r(s_t, a_t) - 100\lambda_{1} \cl(s_t,a_t) - 40\lambda_{2} \cc(s_t,a_t), \label{eq:baselinereward}
% \end{alignat*}
% where $\lambda_{1}, \lambda_{2}\equiv 1$ is the standard RL with fixed weight coefficient combination in prior research~\cite{almasi2020robust}. Further experiment parameters are provided in the Appendix.

% The \drcpo\ algorithm completes the training in approximately 70 hours, reaching convergence in 50,000 episodes.
% The \crcpo\ algorithm completes the training in approximately 150 hours, reaching convergence in 200,000 episodes. The relatively slow training speed is primarily due to the slow data collection in the physical simulator, the large exploration space, and the learning of the Lagrange parameters.

\subsection{Handling illegal driving situations}
\noindent\textbf{Lane Switching Cost:}
We define lane switching cost as a training trick in all continuous settings baselines by quantifying lane switching behaviors with a boolean indicator $\mathds{1}_{\mathrm{swt}}$. This cost helps enforce lane keeping, despite continuous agents' tendency to perform rapid lane switches due to high wheel speeds as Figure~\ref{fig:secondhalf}. Yet the lane deviation constraint fails to inhibit such maneuvers.We measure the lane switching cost, represented by the following equation:
\begin{gather}
    \ci(s,a) = \mathds{1}_{\mathrm{swt}},\\
    \mathds{1}^{\mathrm{swt}} = \left\{
        \begin{aligned}
        &1 && \text{if $d^{\mathrm{lane}}_{t-1}<\beta\cdot d^{\mathrm{center}}$ and $d^{\mathrm{lane}}_{t}>\beta\cdot d^{\mathrm{center}}$;}\\
        &0 && \text{otherwise.}
        \end{aligned}\right.
\end{gather}
where $\beta = 0.9$ is a safety factor and $d^{\mathrm{center}}$ is the midpoint distance of the right lane. $\mathds{1}^{\mathrm{swt}}$ is decided by whether the agent cross the factored central line. We consider $J_{\ci}^{\pi_\theta} = \E [\sum_{t=0}^{H-1} \ci(s_t, a_t) | \pi_\theta] \leq \alpha_3$ as the expected lane switching cost constraint. We omit the lane switching cost in formulation from Section 4.2 as it closely mirrors that of the collision cost, avoiding duplication of similar concepts. This technique is used in our experiments for training purposes and is not applied in discrete settings.

\begin{figure}[t]
    \centering
    \hfill
        \begin{subfigure}[b]{0.22\textwidth}
            \centering
            \resizebox{0.8\textwidth}{!}{\input{figure/illegalaction}}
            \caption{Lane switching behaviour.}
            \label{fig:illegalaction}
        \end{subfigure}
    \hfill
        \hfill
        \begin{subfigure}[b]{0.22\textwidth}
            \centering
            \resizebox{0.9\textwidth}{!}{\input{figure/illegalillustrate.tex}}
            \caption{Lane deviation cost.}
            \label{fig:illegalillustrate}
        \end{subfigure}
        \caption{With the lane switching behavior, the agent under continuous setting can change the lane with small penalties on lane deviation cost at $d^{\mathrm{center}}$.}
        \label{fig:secondhalf}

\end{figure}

%\aea{Why only in continuous and not discrete?Not explained.[Note: done] Also, why is this in Appendix?[Note: page]}

% \subsection{Hardware details of Duckiebot}
% The Duckiebot is equipped with the Jetson Nano hardware, which has one Quad-Core ARM Cortex-A57 64-bit CPU and one NVIDIA Maxwell with 128 CUDA cores GPU. A prevalent autonomous driving functional architecture \cite{velasco2020autonomous} which contains perception, decision, vehicle control, has been built for the Duckiebot on the Robot Operating System (ROS2)\cite{macenski2022robot}
%\aea{citation missing[Re: done]}. 

% \begin{equation}
%     r = distance - w_1 \cdot deviation - w_2 \cdot collision\nonumber
% \end{equation}

\begin{table*}[t]
    \centering
    \caption{Performance comparison of baselines.}
    \begin{tabular}{ccccccccc}
% \toprule
\hlineB{2}
\addlinespace[2pt]
\multirow{2}{*}{\textbf{Scenarios}} & \multirow{2}{*}{\textbf{Metrics}} & \multicolumn{3}{c}{\textbf{Discrete Methods}} & \multicolumn{4}{c}{\textbf{Continuous Methods}} \\
% \cline{3-5} \cline{6-9}
\cmidrule(rl){3-5} \cmidrule(rl){6-9}
\addlinespace[2pt]
 &  & \drcpo & \dppof & \bl~\cite{bellman1952theory} & \crcpo & \cppof & \cbc~\cite{bertesekas1999nonlinear} & \opencv~\cite{chen2020lane}  \\
\midrule
\multirow{3}{*}{Small loop} & Lane Deviation Cost & {0.66$\pm$0.02} & 0.99$\pm$0.07 & 0.98$\pm$0.14 & \textbf{0.31$\pm$0.00} & 1.04$\pm$0.25 & 0.79$\pm$0.02 & 1.65$\pm$0.16\\
                                & Collision Cost & {0.17$\pm$0.00} & 0.38$\pm$0.04 & 0.37$\pm$0.00 & \textbf{0.05$\pm$0.01} & 0.34$\pm$0.20 & 0.17$\pm$0.00 & 0.88$\pm$0.14\\
                                & Travel Distance Reward & \textbf{69.0$\pm$0.6} & 46.6$\pm$3.2 & 50.2$\pm$2.6 & {62.4$\pm$22.2} & 51.3$\pm$14.8 & 43.8$\pm$0.0 & 18.4$\pm$5.1\\
\midrule
\multirow{3}{*}{Zig-zag} & Lane Deviation Cost & {0.57$\pm$0.04} & 0.82$\pm$0.08 & 0.98$\pm$0.02 & \textbf{0.41$\pm$0.02} & 0.86$\pm$0.10 & 0.77$\pm$0.02 & 1.60$\pm$0.10\\
                             & Collision Cost & {0.12$\pm$0.00} & 0.31$\pm$0.02 & 0.41$\pm$0.05 & \textbf{0.06$\pm$0.00} & 0.24$\pm$0.08 & 0.16$\pm$0.04 & 0.87$\pm$0.12\\
                             & Total Distance Reward & \textbf{72.6$\pm$0.1} & 52.3$\pm$6.2 & 46.1$\pm$5.5 & {63.7$\pm$0.5} & 59.3$\pm$6.5 & 49.7$\pm$1.0 & 19.3$\pm$3.8\\
\midrule
\multirow{3}{*}{\makecell{Dynamic obstacle}} & Lane Deviation Cost & {0.63$\pm$0.15} & 0.88$\pm$0.00 & 0.93$\pm$0.18 & \textbf{0.38$\pm$0.08} & 0.64$\pm$0.19 & 0.77$\pm$0.06 & --\\
                             & Collision Cost & {0.32$\pm$0.05} & 0.47$\pm$0.09 & 0.78$\pm$0.12 & \textbf{0.20$\pm$0.08} & 0.33$\pm$0.06 & 0.48$\pm$0.04 & --\\
                             & Total Distance Reward & {68.8$\pm$4.1} & 45.1$\pm$5.6 & 33.0$\pm$5.7 & \textbf{82.0$\pm$16.4} & 63.0$\pm$24.1 & 57.1$\pm$1.0 & --\\
\addlinespace[2pt]
\hlineB{2}
\end{tabular}

    \label{tab:tab_sl_zz}
\end{table*}
